# Supplementary material for: VS-Net: Voting with Segmentation for Visual Localization
Source: arXiv:2105.10886 source file (2021-05-23)
Supplement: Supplementary file 1 [file MapComparison.tex]

\begin{figure}[b]
    \centering
    \includegraphics[width=1.0\linewidth, trim={30mm 70mm 40mm 0mm}, clip]{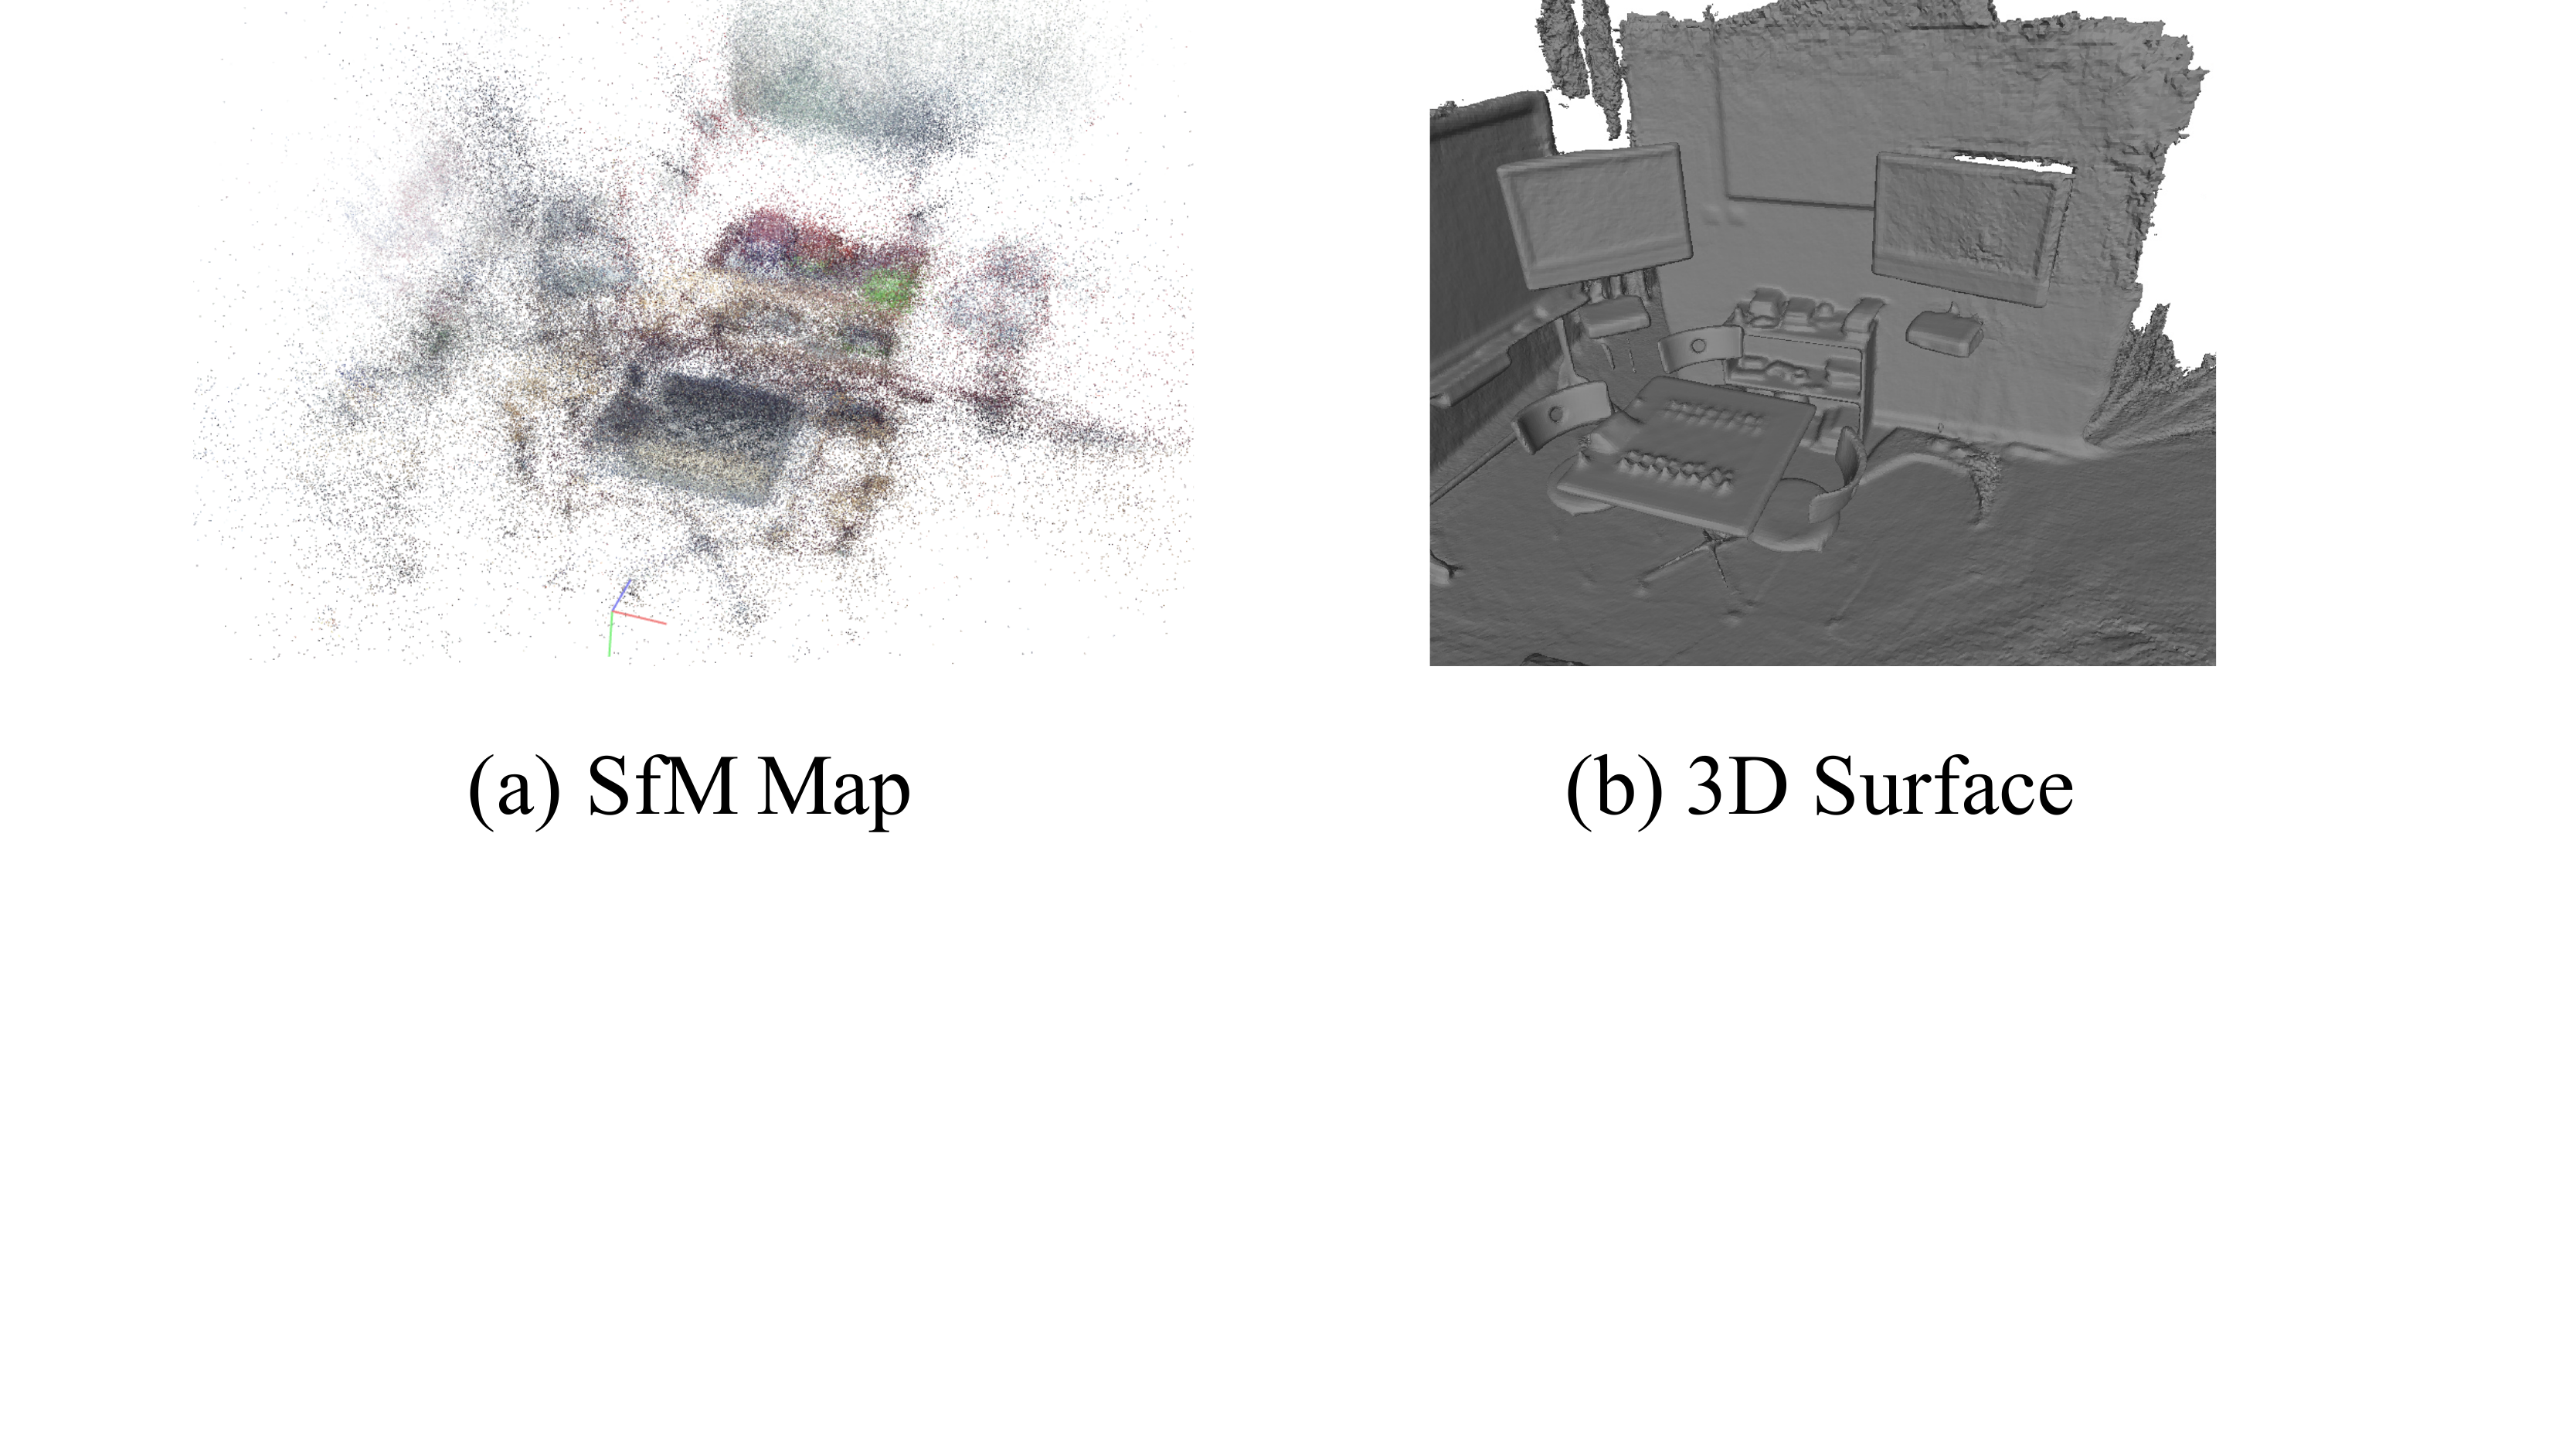}
    \caption{Comparison of (a) SfM feature map and (b) TSDF surface.
    % We compare the SfM feature map and the TSDF surface.
    % (a) is a SIFT feature map built by COLMAP~\cite{}.
    % Classical feature-based visual localization relies on the map reconstructed by SfM, which is typically messy and not accurate enough even in a static indoor scene. 
    % (b) is the map reconstructed from KinectFusion~\cite{} with ToF.
    % The neat and accurate 3D surface can improve the localization accuracy of scene coordinate regression and scene-specific landmarks.
    % The general local features utilized may not best fit a specific scene.
    % (b) Scene coordinate regression trains a neural network to fit the scene and can benefit from high precision surface so that it gets better localization accuracy. The robustness yet is impacted in dynamic environments.
    % Scene-specific landmarks prediction achieves higher accuracy benefiting from the high precision surface. 
    % Meanwhile, it gains higher robustness because the general features may not best fit a specific scene.
    }
    \label{Fig:Map comparison}
\end{figure}
