# Supplementary material for: VS-Net: Voting with Segmentation for Visual Localization
Source: arXiv:2105.10886 source file (2021-05-23)
Supplement: Supplementary file 2 [file street.tex]

\begin{figure}[t]
    \centering
    \includegraphics[width=0.9\linewidth, trim={0 0 0 0}, clip]{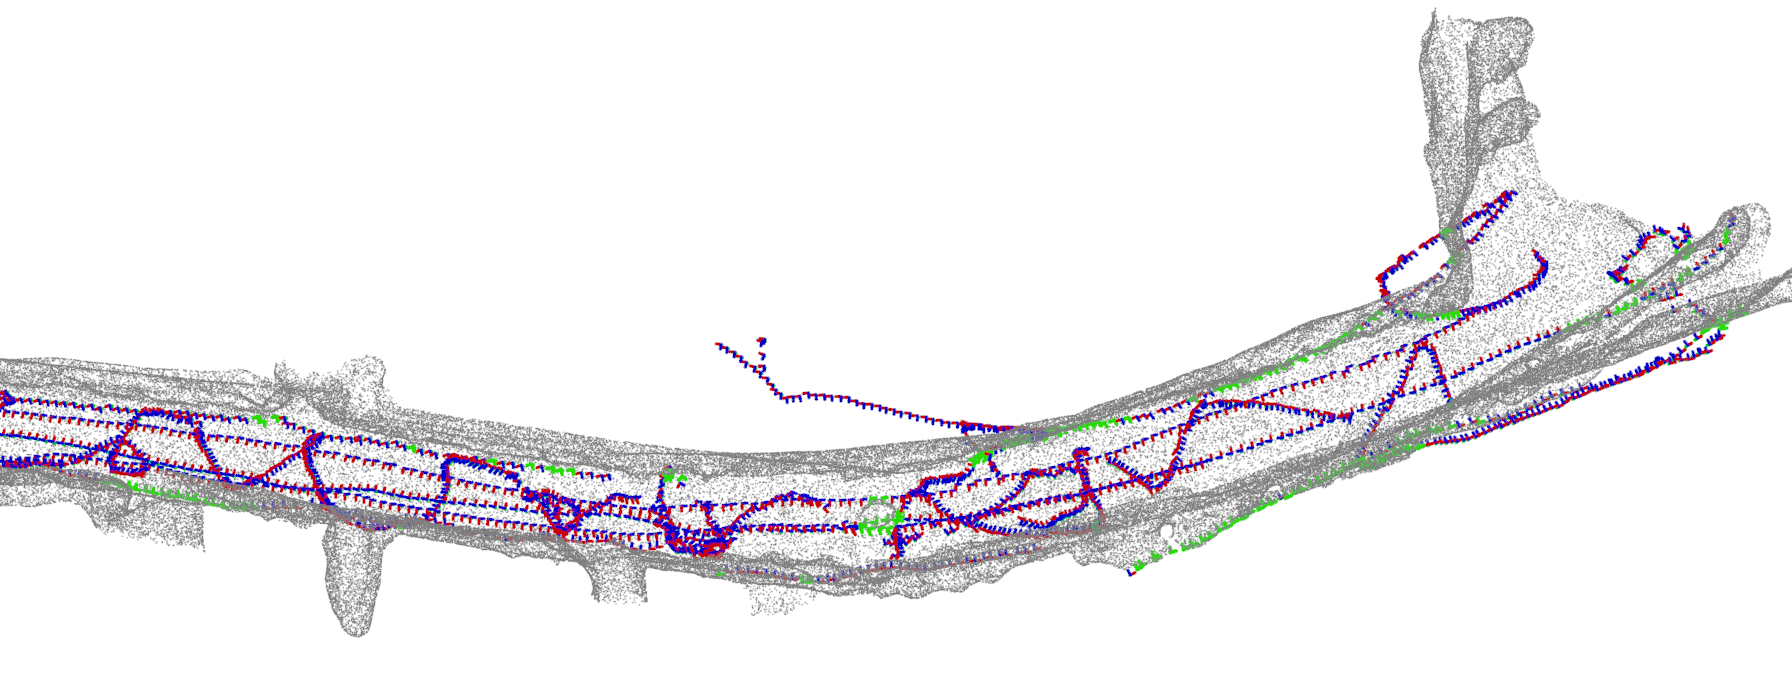}
    \caption{Case study of \textit{Street} in the \textit{Cambridge Landmarks Dataset}.
    % We present a part of the 3D map and the ground-truth camera trajectory of the \textit{Street}.
    % % We present a part of the 3D map we use which is built by multiview stereo and the ground truth camera trajectory of the \textit{Street}.
    % The cameras within 0.5m to the wall are rendered as green.
    % As we can see,
    % the built map is poor, and the ground-truth camera trajectory drifts seriously,
    % which makes the patches and landmarks projected into cameras are highly inconsistent with visual cues.
    % % The same result also happens in DSAC.
    % Active Search~\cite{sattler2012improving} does not require global consistency, so it figures out reasonable results.
    }
    \label{Fig:failure case}
\end{figure}
